# Supplementary material for: Chemo-Mechanical Model of SEI Growth on Silicon Electrode Particles
Source: arXiv:2108.04078 ancillary file (2022-11-30)
Supplement: Supplementary file 1 [file Supporting_Information.pdf]

# Supporting Information: Chemo-Mechanical Model of SEI Growth on Silicon Electrode Particles

Lars von Kolzenberg †‡ Arnulf Latz †‡§

Birger Horstmann *†‡§

November 30, 2022

## 1 Theory

This section describes the derivation of a thermodynamically consistent theory for the chemo-mechanical coupling inside expanding electrode particles with a surrounding SEI. Figure 1 schematically depicts the deformation of the system. The deformation gradient $\mathbf{F} = \partial\vec{x}/\partial\vec{X}_0$ relates the Lagrangian domain $\Omega_0$ to the Eulerian domain $\Omega$ with the volume expansion $\det\mathbf{F} = J = V/V_0$ [1]. For this Lagrangian frame, we derive a general thermodynamic consistent theory in the next section. Based on this formalism, we then proceed to derive a model for the electrode particle and the SEI.

*Corresponding Author: birger.horstmann@dlr.de

†German Aerospace Center, Pfaffenwaldring 38-40, 70569 Stuttgart, Germany

‡Helmholtz Institute Ulm, Helmholtzstraße 11, 89081 Ulm, Germany

§Ulm University, Albert-Einstein-Allee 47, 89081 Ulm, Germany

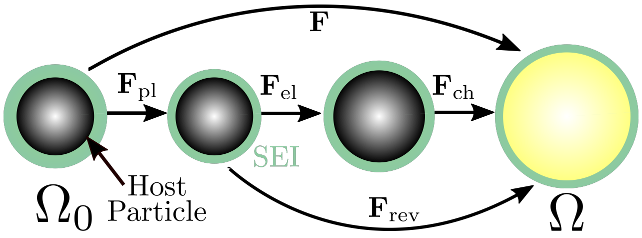


Figure 1: Schematic representation of particle and SEI deformation. The compound deforms plastically $\mathbf{F}_{\text{pl}}$, elastically $\mathbf{F}_{\text{el}}$, and finally chemically $\mathbf{F}_{\text{ch}}$.

## 1.1 Thermodynamic consistent Theory

In this section, we derive a thermodynamically consistent model for mobile species in a host material [2, 3, 4]. As shown in Figure 1, different effects deform the host from its initial Lagrangian geometry $\Omega_0$ to the current Eulerian geometry $\Omega$. During the deformation, the overall mass of the particle changes due to a change of mobile species concentration. We avoid the influences from changing total mass and changing geometry by stating our balances in the Lagrangian frame "0" and defining all quantities relative to the constant host mass "H".

An arbitrary intensive quantity $\psi$ changes over time due to a flux $\vec{N}_\psi$ across the boundary and source terms $B_\psi$ inside the volume according to the integral balance SI-1,

$$\frac{\mathrm{d}}{\mathrm{d}t}\int_V \psi \mathrm{d}V = -\oint_{\partial V} \vec{N}_\psi \mathrm{d}A + \int B_\psi \mathrm{d}V. \tag{SI-1}$$

We define the volume specific quantities as host mass specific quantities, $\psi = \rho_\mathrm{H}\psi_\mathrm{H}$,$B_\psi = \rho_\mathrm{H} B_{\psi,\mathrm{H}}$. Moreover, we take the host material to be the basis for our integral, so that the infinitesimal volumes are host volumes $V = V_\mathrm{H}$. We use the Piola transformation to transform the infinitesimal elements from the Eulerian to the Lagrangian frame of reference

$$\begin{aligned}\frac{\mathrm{d}}{\mathrm{d}t}\int_{V_{\mathrm{H},0}} \rho_{\mathrm{H},0}\psi_\mathrm{H} \mathrm{d}V_{\mathrm{H},0} = &-\oint_{\partial V_{\mathrm{H},0}} J\vec{N}_{\psi,\mathrm{H}}\mathbf{F}^{-\mathsf{T}}\mathrm{d}A_{\mathrm{H},0} \\ &+ \int \rho_{\mathrm{H},0} B_{\psi,\mathrm{H}} \mathrm{d}V_{\mathrm{H},0}.\end{aligned} \tag{SI-2}$$

Here we introduced the deformation tensor $\mathbf{F}$, which relates the Lagrangian domain $\Omega_0$ to the Eulerian domain $\Omega$ according to Figure 1. Its determinant $\det\mathbf{F} = J = V_\mathrm{H}/V_{\mathrm{H},0}$ determines the volume expansion. Additionally, we introduced the constant Lagrangian host density $\rho_{\mathrm{H},0} = \rho_\mathrm{H}/J$. Finally, we apply Gauss's theorem and obtain the differential balance in the Lagrangian frame

$$\rho_{\mathrm{H},0}\dot{\psi}_\mathrm{H} = -\nabla_0\cdot\vec{N}_{\psi,\mathrm{H},0} + \rho_{\mathrm{H},0}B_{\psi,\mathrm{H}}. \tag{SI-3}$$

Here, $\dot{\psi}_\mathrm{H} = \frac{\partial\psi_\mathrm{H}}{\partial t} + \vec{v}_\mathrm{H}\nabla\cdot\psi_\mathrm{H}$ is the material derivative in the host frame with the host velocity $\vec{v}_\mathrm{H}$.

We start the derivation of our model by balancing the lithium concentration $c_{\mathrm{Li},0}$ inside the host material with the continuity Equation SI-4,

$$\dot{c}_{\mathrm{Li},0} = -\nabla_0\cdot\vec{N}_{\mathrm{Li},0}. \tag{SI-4}$$

The host-relative flux is defined as the difference between lithium and host velocity $\vec{N}_{\mathrm{Li},0} = c_{\mathrm{Li},0}\left(\vec{v}_\mathrm{Li} - \vec{v}_\mathrm{H}\right)$. Next we balance the momentum $\vec{g}$ with Equation SI-5,

$$\rho_{\mathrm{H},0}\dot{\vec{g}}_\mathrm{H} = \nabla_0\cdot\mathbf{P} + \rho_{\mathrm{H},0}\vec{b}_\mathrm{H}. \tag{SI-5}$$

Here, $\mathbf{P} = \det(\mathbf{F})\sigma\mathbf{F}^{-\mathsf{T}}$ denotes the first Piola–Kirchhoff stress tensor, which is the Piola transformation of the Cauchy stress $\sigma$ to the reference configuration.

Additionally, the momentum changes due to body forces $\vec{b}_{\mathrm{H}}$ inside the host frame, *e.g.* gravity.

The total energy density $e$ in our isothermal system changes according to Equation SI-6,

$$\rho_{\mathrm{H},0}\dot{e}_{\mathrm{H}} = \rho_{\mathrm{H},0}\vec{v}_{\mathrm{H}}\vec{b}_{\mathrm{H}} + \nabla_0\cdot\left(\mathbf{P}^{\mathsf{T}}\vec{v}_{\mathrm{H}}\right). \tag{SI-6}$$

We express the body forces $\vec{b}_{\mathrm{H}}$ with the momentum balance SI-5 and apply the product rule $\nabla_0\cdot\left(\mathbf{P}^{\mathsf{T}}\vec{v}_{\mathrm{H}}\right) = \vec{v}_{\mathrm{H}}\nabla_0\cdot\mathbf{P} + \mathbf{P}\colon\nabla_0\vec{v}_{\mathrm{H}}$. Here $\mathbf{A}\colon\mathbf{B} = \sum_{i,j} a_{i,j}b_{i,j}$ denotes the double contraction of two tensors. Moreover, we use the identity $\dot{\mathbf{F}} = \nabla_0\vec{v}_{\mathrm{H}}$ to obtain the following expression for the change in internal energy $\dot{u}_{\mathrm{H}} = \dot{e}_{\mathrm{H}} - \vec{v}_{\mathrm{H}}\dot{\vec{g}}_{\mathrm{H}}$,

$$\rho_{\mathrm{H},0}\dot{u}_{\mathrm{H}} = \mathbf{P}\colon\dot{\mathbf{F}}. \tag{SI-7}$$

The second law of thermodynamics imposes a non-negative dissipation rate $\mathcal{R} \geq 0$ and thereby constrains the form of thermodynamic consistent constitutive equations. To obtain a dissipation equation, we state a generic isothermal balance of the entropy $s$,

$$\rho_{\mathrm{H},0}T\dot{s}_{\mathrm{H}} = -\nabla_0\cdot T\vec{N}_{\mathrm{S},0} + \mathcal{R}, \tag{SI-8}$$

with the entropy flux $\vec{N}_{\mathrm{S},0}$, which we identify in the following. We write Equation SI-8 in terms of the free energy $\varphi_{\mathrm{H}}$ using the Legendre-transformation of the internal energy $\varphi_{\mathrm{H}} = u_{\mathrm{H}} - Ts_{\mathrm{H}}$ with

$$\mathcal{R} = -\rho_{\mathrm{H},0}\dot{\varphi}_{\mathrm{H}} + \mathbf{P}\colon\dot{\mathbf{F}} + \nabla_0\cdot T\vec{N}_{\mathrm{S},0} \geq 0. \tag{SI-9}$$

The total time derivative of the free energy of a mobile species in an elastic material is defined by

$$\rho_{\mathrm{H},0}\dot{\varphi}_{\mathrm{H}} = \mu_{\mathrm{Li}}\dot{c}_{\mathrm{Li},0} + \frac{1}{2}\mathbf{T}_{\mathrm{rev}}\colon\dot{\mathbf{C}}_{\mathrm{rev}} \tag{SI-10}$$

with the reversible right Cauchy-Green tensor $\mathbf{C}_{\mathrm{rev}} = \mathbf{F}_{\mathrm{rev}}^{\mathsf{T}}\mathbf{F}_{\mathrm{rev}}$. Equation SI-10 directly yields the following constitutive equations to determine the chemical potential $\mu_{\mathrm{Li}}$ and the reversible second Piola–Kirchhoff stress tensor $\mathbf{T}_{\mathrm{rev}} = J\mathbf{F}_{\mathrm{rev}}^{-1}\sigma\mathbf{F}_{\mathrm{rev}}^{-\mathsf{T}}$,

$$\mu_{\mathrm{Li}} = \frac{\partial\left(\rho_{\mathrm{H},0}\varphi_{\mathrm{H}}\right)}{\partial c_{\mathrm{Li},0}}, \tag{SI-11}$$

$$\mathbf{T}_{\mathrm{rev}} = 2\frac{\partial\left(\rho_{\mathrm{H},0}\varphi_{\mathrm{H}}\right)}{\partial\mathbf{C}_{\mathrm{rev}}}. \tag{SI-12}$$

Inserting the free energy density SI-10 into the dissipation Equation SI-9 yields

$$\mathcal{R} = -\mu_{\mathrm{Li}}\dot{c}_{\mathrm{Li},0} - \frac{1}{2}\mathbf{T}_{\mathrm{rev}}\colon\dot{\mathbf{C}}_{\mathrm{rev}} + \mathbf{P}\colon\dot{\mathbf{F}} + \nabla_0\cdot T\vec{N}_{\mathrm{S},0} \geq 0. \tag{SI-13}$$

We identify the entropy flux as $\vec{N}_{\mathrm{S},0} = (\mu_{\mathrm{Li}}\vec{N}_{\mathrm{Li},0})/T$ using the continuity Equation SI-4 with $\mu_{\mathrm{Li}}\nabla_0\cdot\vec{N}_{\mathrm{Li},0} = \nabla_0\cdot\mu_{\mathrm{Li}}\vec{N}_{\mathrm{Li},0} - \vec{N}_{\mathrm{Li},0}\nabla_0\mu_{\mathrm{Li}}$. The mechanical power

density $\mathbf{P} : \dot{\mathbf{F}}$ consists of a reversible and an irreversible part according to Section SI-3,

$$\mathbf{P} : \dot{\mathbf{F}} = \frac{1}{2}\mathbf{T}_{\text{rev}} : \dot{\mathbf{C}}_{\text{rev}} + \mathbf{M} : \mathbf{L}_{\text{pl}}. \tag{SI-14}$$

Here we introduced the Mandel stress $\mathbf{M} = \mathbf{C}_{\text{rev}}\mathbf{T}_{\text{rev}}$ and the plastic velocity gradient $\mathbf{L}_{\text{pl}} = \dot{\mathbf{F}}_{\text{pl}}\mathbf{F}_{\text{pl}}^{-1}$ [5, 6]. With these considerations, we obtain the final expression for the dissipation rate,

$$\mathcal{R}_0 = -\vec{N}_{\text{Li},0} \cdot \nabla_0 \cdot \mu_{\text{Li}} + \mathbf{M} : \mathbf{L}_{\text{pl}} \geq 0. \tag{SI-15}$$

Building on this general framework, we derive constitutive equations for the electrode particle and the surrounding SEI in the next two subsections.

## 1.2 Electrode Particle Model

We apply the previously introduced general framework in this section to model an electrode particle. We neglect plastic deformations of the host material so that the overall deformation is completely reversible. The reversible deformation consists of an elastic part $\mathbf{F}_{\text{el}}$ due to mechanical stress and a chemical part $\mathbf{F}_{\text{ch}}$ coming from changes in lithium concentration

$$\mathbf{F} = \mathbf{F}_{\text{rev}} = \mathbf{F}_{\text{el}}\mathbf{F}_{\text{ch}}. \tag{SI-16}$$

The chemical deformation is isotropic and the particle volume increases linearly with lithium concentration $c_{\text{Li},0}$ according to

$$J_{\text{ch}} = 1 + v c_{\text{Li},0} = \lambda_{\text{ch}}^3 = \det \mathbf{F}_{\text{ch}}, \qquad \mathbf{F}_{\text{ch}} = \lambda_{\text{ch}}\mathbf{Id}. \tag{SI-17}$$

with the molar volume $v$ of lithium inside the host [7].

We couple chemistry and mechanics with the free energy density in the Lagrangian frame $\rho_{\text{H},0}\varphi_{\text{H}}$ from which we subsequently derive our set of constitutive equations.

$$\rho_{\text{H},0}\varphi_{\text{H}} = \rho_{\text{H},0}\varphi_{\text{H,ch}}(c_{\text{Li}}) + \rho_{\text{H},0}\varphi_{\text{H,el}}(\mathbf{F}_{\text{el}}, c_{\text{Li}}). \tag{SI-18}$$

For the chemical part of the free energy, we rely on experimentally obtained open circuit voltage (OCV) curves $U_0(c_{\text{Li}})$ [3, 8, 9, 10]

$$\rho_{\text{H},0}\varphi_{\text{H,ch}}(c_{\text{Li}}) = -\int_0^{c_{\text{Li}}} F U_0(c'_{\text{Li}}) \mathrm{d}c'_{\text{Li}}. \tag{SI-19}$$

For the elastic part of the free energy $\varphi_{\text{H,el}}$, we take a linear elastic model

$$\rho_{\text{H},0}\varphi_{\text{H,el}} = \frac{1}{2}\left[\lambda_{\text{H}} \left(\text{tr}\left(\mathbf{E}_{\text{el}}\right)\right)^2 + 2G_{\text{H}} \,\text{tr}\left(\mathbf{E}_{\text{el}}^2\right)\right] \tag{SI-20}$$

using the first and second Lamé constants $\lambda_{\text{H}} = 2G_{\text{H}}\nu_{\text{H}}/(1 - 2\nu_{\text{H}})$ and $G_{\text{H}} = E_{\text{H}}/2(1 + \nu_{\text{H}})$ with Young's modulus $E_{\text{H}}$ and Poisson's ratio $\nu_{\text{H}}$. The elastic

strain depends on the elastic right Cauchy–Green tensor $\mathbf{C}_{\mathrm{el}} = \mathbf{F}_{\mathrm{el}}^{\mathsf{T}}\mathbf{F}_{\mathrm{el}}$ according to Equation SI-21,

$$\mathbf{E}_{\mathrm{el}} = \frac{1}{2}\left(\mathbf{C}_{\mathrm{el}} - \mathbf{Id}\right) = \frac{1}{2}\left(\lambda_{\mathrm{ch}}^{-2}\mathbf{C} - \mathbf{Id}\right). \tag{SI-21}$$

We use the definitions SI-11 and SI-12 to derive the stress and the chemical potential

$$\mathbf{P} = 2\mathbf{F}\frac{\partial \rho_{\mathrm{H},0}\varphi_{\mathrm{H}}}{\partial \mathbf{C}} = \lambda_{\mathrm{ch}}^{-2}\mathbf{F}\left(\lambda_{\mathrm{H}}\,\mathrm{tr}(\mathbf{E}_{\mathrm{el}})\mathbf{Id} + 2G_{\mathrm{H}}\mathbf{E}_{\mathrm{el}}\right) \tag{SI-22}$$

$$\mu_{\mathrm{Li}} = \frac{\partial \rho_{\mathrm{H},0}\varphi_{\mathrm{H}}}{\partial c_{\mathrm{Li},0}} = -FU_0 - \frac{v}{3J_{\mathrm{ch}}}\mathbf{P} : \mathbf{F}. \tag{SI-23}$$

With these definitions, we model the transient chemo-mechanical coupling. We specify the lithium flux of Equation SI-24 in line with the dissipation inequality SI-15 to guarantee positive entropy production. For the elastic deformation, we use the momentum balance (see Equation SI-25) and neglect body $\vec{b}_{\mathrm{H}} = 0$ and inertial forces $\dot{\vec{g}}_{\mathrm{H}} = 0$. This leads to the following differential algebraic equations (DAE),

$$\dot{c}_{\mathrm{Li},0} = -\nabla_0 \cdot \vec{N}_{\mathrm{Li},0} \quad \text{with} \quad \vec{N}_{\mathrm{Li},0} = -L\nabla_0 \mu_{\mathrm{Li}}, \tag{SI-24}$$

$$0 = \nabla_0 \cdot \mathbf{P}. \tag{SI-25}$$

Here the mobility $L$ is proportional to the diffusion constant $D_{\mathrm{Li}}$ by $L = D_{\mathrm{Li}}(\partial \mu_{\mathrm{Li}}/\partial c_{\mathrm{Li},0})^{-1}$.

## 1.3 SEI Model

In this section, we derive a model for coupled SEI growth and mechanics. We model the SEI as porous medium consisting of an incompressible SEI matrix and electrolyte inside its pores, as introduced by Single *et al.* [11, 12]. The volume fractions $\epsilon_{\mathrm{SEI}} = V_{\mathrm{SEI}}/V$ and $\epsilon_{\mathrm{elyt}} = V_{\mathrm{elyt}}/V = 1 - \epsilon_{\mathrm{SEI}}$ characterize the macroscopic composition at each point. The macroscopic deformation tensor $\bar{\mathbf{F}}$ describes the overall volume deformation and consists of three parts

$$\bar{\mathbf{F}} = \bar{\mathbf{F}}_{\mathrm{el}}\bar{\mathbf{F}}_{\mathrm{pl}}\bar{\mathbf{F}}_{\mathrm{ref}}. \tag{SI-26}$$

The first part is a reference deformation $\bar{\mathbf{F}}_{\mathrm{ref}}$, which we introduce to set the stress free SEI configuration for healing SEI elements. Additionally the SEI deforms plastically $\bar{\mathbf{F}}_{\mathrm{pl}}$ and finally elastically $\bar{\mathbf{F}}_{\mathrm{el}}$.

### SEI Growth

The SEI grows continuously over time, as electrons $e^-$, lithium ions $Li^+$ and electrolyte molecules coincide. We simplify the multitude of possible SEI growth reactions to the formation of the most prominent SEI component $Li_2EDC$ from EC, reaction SI-27

$$2\mathrm{Li}^0 + 2\mathrm{EC} \rightarrow \mathrm{Li_2EDC} + \mathrm{R}. \tag{SI-27}$$

Here R is a gaseous residue and $\mathrm{Li}^0 = \mathrm{Li}^+ + \mathrm{e}^-$ are lithium ions with coordinated electrons, forming neutral lithium interstitial atoms [13, 14, 15, 16]. We use Equation SI-27 to describe the SEI formation reaction kinetic,

$$r_{\mathrm{SEI}} = k c_{\mathrm{Li}^0}^2, \tag{SI-28}$$

with the lithium atom concentration $c_{\mathrm{Li}^0}$ inside the SEI and the rate constant $k$. Here, we assumed a constant electrolyte concentration.

The concentration of lithium atoms in the SEI changes over time due to an interstitial flux $\vec{N}_{\mathrm{Li}^0}$ and the SEI formation reaction SI-27 according to the integral balance SI-29

$$\frac{\mathrm{d}}{\mathrm{d}t} \int c_{\mathrm{Li}^0} \mathrm{d}V_{\mathrm{SEI}} = -\oint \vec{N}_{\mathrm{Li}^0} \mathrm{d}A_{\mathrm{SEI}} - 2 \int r_{\mathrm{SEI}} \Gamma A_{\mathrm{V}} \mathrm{d}V \tag{SI-29}$$

with the surface site density $\Gamma$. For the specific surface $A_{\mathrm{V}}$ we rely on the model of Single *et al.* [11, 12] and adapt it to a spherical symmetric geometry

$$A_{\mathrm{V}} = 6 a_0 \epsilon_{\mathrm{elyt}} \left( \epsilon_{\mathrm{SEI}} + \frac{1}{6} a_0^2 \left( \frac{\partial^2 \epsilon_{\mathrm{SEI}}}{\partial R^2} + \frac{2}{R} \frac{\partial \epsilon_{\mathrm{SEI}}}{\partial R} + \frac{\epsilon_{\mathrm{SEI}}}{2R^2} \right) \right) \tag{SI-30}$$

with the characteristic pore size $a_0$, see Section SI-4. We transform Equation SI-29 into a differential balance using the Piola transformation and Gauss's theorem

$$\frac{\mathrm{d}(\epsilon_{\mathrm{SEI}} c_{\mathrm{Li}^0,0})}{\mathrm{d}t} = -\epsilon_{\mathrm{SEI}} \nabla_0 \cdot \vec{N}_{\mathrm{Li}^0,0} - 2 \bar{J} r_{\mathrm{SEI}} \Gamma A_{\mathrm{V}}. \tag{SI-31}$$

We determine the flux with Fick's law $\vec{N}_{\mathrm{Li}^0,0} = -D_{\mathrm{Li}^0} \nabla_0 c_{\mathrm{Li}^0,0}$ with the diffusivity $D_{\mathrm{Li}^0}$ of lithium atoms inside the SEI [17]. The Lagrangian SEI porosity $\varepsilon_{\mathrm{SEI},0} = \bar{J} \epsilon_{\mathrm{SEI}}$ changes over time as new SEI forms according to

$$\frac{\mathrm{d}}{\mathrm{d}t} \int \mathrm{d}V_{\mathrm{SEI}} = \int r_{\mathrm{SEI}} \Gamma A_{\mathrm{V}} \bar{V}_{\mathrm{SEI}} \mathrm{d}V \tag{SI-32}$$

with the average molar volume of SEI components $\bar{V}_{\mathrm{SEI}}$. Applying the Piola transformation leads to the following differential balance for the SEI volume fraction

$$\dot{\varepsilon}_{\mathrm{SEI},0} = \bar{J} r_{\mathrm{SEI}} \Gamma A_{\mathrm{V}} \bar{V}_{\mathrm{SEI}}. \tag{SI-33}$$

### SEI Mechanics

The SEI deforms elastoplastically until it eventually fractures as the electrode particle beneath expands and contracts. We determine the elastic deformation with the momentum balance inside the SEI

$$\nabla_0 \cdot \mathbf{P}_{\mathrm{SEI}} = 0, \tag{SI-34}$$

where we again neglect inertial and body forces. We derive an expression for the elastic stress from the micromechanical model stated by Danielsson *et al.*

[18]. In their model, they derive an elastic free energy in a porous medium, which is subject to purely elastic deformation. Because our SEI also deforms plastically, we state their free energy in the plastically deformed intermediate configuration $\Omega_{\mathrm{pl}} = \bar{\mathbf{F}}_{\mathrm{pl}}\bar{\mathbf{F}}_{\mathrm{ref}}\Omega_0$. Accordingly, we use the porosity $\varepsilon_{\mathrm{pl}} = 1 - (1-\epsilon_{\mathrm{elyt}})/(\bar{J}_{\mathrm{pl}}\bar{J}_{\mathrm{ref}})$ and transform the free energy to the Lagrange frame with $\rho_{\mathrm{H},0}\varphi_{\mathrm{H}} = \bar{J}_{\mathrm{pl}}\bar{J}_{\mathrm{ref}}\rho_{\mathrm{H,pl}}\varphi_{\mathrm{H}}$. We express the energy only in terms of the elastic invariants $\bar{I}_{1,\mathrm{el}} = \operatorname{tr}\bar{\mathbf{C}}_{\mathrm{el}}$ and $\bar{J}_{\mathrm{el}} = \sqrt{\det\bar{\mathbf{C}}_{\mathrm{el}}}$.

$$\rho_{\mathrm{SEI},0}\varphi_{\mathrm{SEI,el}} = \bar{J}_{\mathrm{pl}}\bar{J}_{\mathrm{ref}}\frac{G}{2} \cdot \left[\bar{I}_{1,\mathrm{el}}\left(2 - \frac{1}{\bar{J}_{\mathrm{el}}} - \frac{\varepsilon_{\mathrm{pl}} + 2(\bar{J}_{\mathrm{el}}-1)}{\bar{J}_{\mathrm{el}}^{2/3}\eta^{1/3}}\right) - 3(1-\varepsilon_{\mathrm{pl}})\right] \tag{SI-35}$$

$$\eta = 1 + \frac{\bar{J}_{\mathrm{el}}-1}{\varepsilon_{\mathrm{pl}}}. \tag{SI-36}$$

Taking the derivative of this potential with respect to the reversible right Cauchy–Green tensor $\bar{\mathbf{C}}_{\mathrm{rev}} = \bar{\mathbf{C}}_{\mathrm{el}}$ yields an expression for the reversible second Piola–Kirchhoff stress inside the SEI $\mathbf{T}_{\mathrm{SEI,rev}} = 2\partial(\rho_{\mathrm{SEI},0}\varphi_{\mathrm{SEI}})/\partial\bar{\mathbf{C}}_{\mathrm{rev}}$, according to Equation SI-12.

$$\mathbf{T}_{\mathrm{SEI,rev}} = \frac{J_{\mathrm{pl}}J_{\mathrm{ref}}G}{2}\left[\left(4 - \frac{2}{\bar{J}_{\mathrm{el}}} - 2\frac{\varepsilon_{\mathrm{pl}} + 2(\bar{J}_{\mathrm{el}}-1)}{\bar{J}_{\mathrm{el}}^{2/3}\eta^{1/3}}\right)\mathbf{Id} + \bar{J}_{\mathrm{el}}\bar{I}_{1,\mathrm{el}}\left(\frac{1}{\bar{J}_{\mathrm{el}}^2} - \frac{1}{3\bar{J}_{\mathrm{el}}^{2/3}\eta^{1/3}}\frac{(4-\varepsilon_{\mathrm{pl}})\eta + (1-\varepsilon_{\mathrm{pl}})}{\varepsilon_{\mathrm{pl}}\eta^2 + (1-\varepsilon_{\mathrm{pl}})\eta}\right)\bar{\mathbf{C}}_{\mathrm{el}}^{-1}\right] \tag{SI-37}$$

From Equation SI-37 we obtain the first Piola-Kirchhoff stress with the transformation $\mathbf{P}_{\mathrm{SEI}} = \mathbf{F}_{\mathrm{rev}}\mathbf{T}_{\mathrm{SEI,rev}}\mathbf{F}_{\mathrm{pl}}^{-\mathsf{T}}$.

Based on this stress, we proceed to develop a model for plastic deformation and fracture of the SEI. For the plastic deformation we introduce the yield function $f$, which tends to zero if the SEI reaches its yield criterion. The fracture depends on the damage variable $\xi$, which describes the degree of deterioration and reaches from 0 (intact) to 1 (broken). We couple the damage variable to the yield function with the Gurson-Tvergaard-Needleman approach [19, 20, 21, 22]

$$f = \frac{\frac{3}{2}\left|\mathbf{M}_{\mathrm{c}}^{\mathrm{dev}}\right|^2}{\sigma_{\mathrm{Y}}^2} + 2\xi\cosh\left(\frac{1}{2}\frac{\operatorname{tr}(\mathbf{M}_{\mathrm{c}})}{\sigma_{\mathrm{Y}}}\right) - 1 - \xi^2 \leq 0. \tag{SI-38}$$

Here $\mathbf{M}_{\mathrm{c}}^{\mathrm{dev}} = \mathbf{M}_{\mathrm{c}} - 1/3\operatorname{tr}\mathbf{M}_{\mathrm{c}}$ is the deviatoric part of the adapted Mandel stress $\mathbf{M}_{\mathrm{c}} = \mathbf{F}_{\mathrm{rev}}^{\mathsf{T}}\sigma\mathbf{F}_{\mathrm{rev}}^{-\mathsf{T}}$ inside the SEI and $\sigma_{\mathrm{Y}}$ is the yield stress [5, 6, 23]. The damage variable $\xi$ depends on the SEI porosity $\epsilon_{\mathrm{elyt}}$ by Equation SI-39 [22].

$$\xi = \begin{cases} \epsilon_{\mathrm{elyt}} & \text{if } \epsilon_{\mathrm{elyt}} < \epsilon_{\mathrm{elyt,crit}} \\ \epsilon_{\mathrm{elyt}} + (1-\epsilon_{\mathrm{elyt}})\cdot\left(\frac{\epsilon_{\mathrm{elyt}} - \epsilon_{\mathrm{elyt,crit}}}{\epsilon_{\mathrm{elyt,frac}} - \epsilon_{\mathrm{elyt,crit}}}\right) & \text{else.} \end{cases} \tag{SI-39}$$

The critical SEI porosity $\epsilon_{\mathrm{elyt,crit}}$ accounts for pore coalescence, which accelerates mechanical degradation, if the SEI porosity is above the critical porosity

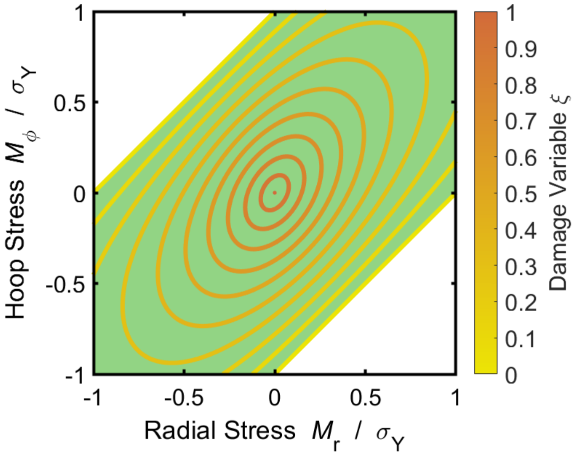


Figure 2: Representation of elastic, plastic and broken regimes in mechanical model. Yield surface $f = 0$ for different degrees $\xi$ of damage. The elastic regime for the undamaged case $\xi = 0$ is colored in green. With increasing damage $\xi$, the surface shrinks until it converges to $(0, 0)$ if SEI is broken $\xi = 1$.

$\epsilon_{\text{elyt}} > \epsilon_{\text{elyt,crit}}$. The fracture SEI porosity $\epsilon_{\text{elyt,frac}}$ describes the porosity at which the SEI ultimately breaks with $\xi(\epsilon_{\text{elyt}} \geq \epsilon_{\text{elyt,frac}}) = 1$.

In Figure 2, we show the yield surface $f = 0$, at which the SEI flows plastically. We observe the classical von-Mises yield surface for $\xi = 0$, which withstands arbitrary large hydrostatic stress and only depends on the deviatoric stress. Damage causes the yield surface to shrink until it converges to the stress $(0, 0)$ for $\xi = 1$.

To describe the plastic flow upon reaching this yield surface, we rely on the maximum plastic dissipation postulate [5, 6, 24, 25, 26, 27] as additional restriction to the principle of positive dissipation, Equation SI-15. This postulate from plasticity theory constraints plastic flow to the normal direction of the yield surface $\partial f / \partial_{\text{c}}$ and thus leads to the following constitutive equation [5, 6],

$$\mathbf{L}_{\text{pl}} = \phi \frac{\partial f}{\partial \mathbf{M}_{\text{c}}}, \tag{SI-40}$$

where the plastic multiplier $\phi$ is non-negative, $\phi \geq 0$, guaranteeing non-negativity of the dissipation rate in Equation SI-15. The plastic multiplier and the yield function $f$ additionally obey the Karush-Kuhn-Tucker condition $\phi f = 0$ [6]. Thus, plastic flow is suppressed $\phi = 0$ during elastic deformation, $f < 0$. For plastic deformation, $f = 0$, $\phi$ results from the consistency condition $\dot{f} = 0$ [6]. Note that the plastic flow is not trace-free and thus not volume preserving, because the yield criterion, Equation SI-38 depends on the hydrostatic stress $\text{tr}\left(_{\text{c}}\right)/3$.

Table SI-1: Dimensionless variables of our model

| | | | | |
|---|---|---|---|---|
| Electrode | | | | |
| $\tilde{R} = \frac{R}{R_0}$ | $\tilde{r} = \frac{r}{R_0}$ | $\tilde{t} = \frac{t}{t_{\mathrm{cycle}}}$ | $\tilde{c} = \frac{c_{\mathrm{Li},0}}{c_{\mathrm{max}}}$ | $\tilde{\mu} = \frac{\mu_{\mathrm{Li}}}{R_{\mathrm{gas}}T}$ |
| $\tilde{U}_0 = \frac{FU_0}{R_{\mathrm{gas}}T}$ | $\tilde{\mathbf{P}} = \frac{\mathbf{P}}{E_{\mathrm{H}}}$ | $\tilde{E}_{\mathrm{H}} = \frac{E_{\mathrm{H}}}{R_{\mathrm{gas}}Tc_{\mathrm{max}}}$ | $\mathrm{Fo} = \frac{D_{\mathrm{Li}}t_{\mathrm{cycle}}}{R_0^2}$ | |
| SEI | | | | |
| $\tilde{c}_{\mathrm{Li}^0} = \frac{c_{\mathrm{Li}^0}}{c_{\mathrm{Li}^0,\mathrm{ref}}}$ | $\tilde{\mathbf{P}}_{\mathrm{SEI}} = \frac{\mathbf{P}}{E_{\mathrm{SEI}}}$ | $\tilde{\mathbf{M}}_{\mathrm{c}} = \frac{\mathbf{M}_{\mathrm{c}}}{\sigma_{\mathrm{Y}}}$ | $\tilde{A}_{\mathrm{V}} = \frac{A_{\mathrm{V}}}{a_0}$ | $\tilde{V} = \bar{V}_{\mathrm{SEI}}c_{\mathrm{Li}^0,\mathrm{ref}}$ |
| $\tilde{\eta}_{\mathrm{int}} = \frac{F\eta_{\mathrm{int}}}{R_{\mathrm{gas}}T}$ | $\tilde{\phi} = \frac{\phi t_{\mathrm{cycle}}}{\sigma_{\mathrm{Y}}}$ | $\mathrm{Fo}_{\mathrm{SEI}} = \frac{D_{\mathrm{Li}^0}t_{\mathrm{cycle}}}{R_0^2}$ | $\mathrm{Da} = \frac{R_0^2 k\Gamma c_{\mathrm{Li}^0,\mathrm{ref}}}{D_{\mathrm{Li}^0}a_0}$ | |

## 1.4 Model Summary

At this point, we recapture and nondimensionalize the equations for the electrode particle and the SEI and introduce appropriate boundary conditions. For this purpose, we choose a spherical symmetric geometry and reduce the model to the radial dimension. The resulting deformation tensor is isotropic,

$$\mathbf{F} = \begin{pmatrix} \partial r/\partial R & 0 & 0 \\ 0 & r/R & 0 \\ 0 & 0 & r/R \end{pmatrix} \tag{SI-41}$$

with the Eulerian radial coordinate $r$ and the Lagrangian radial coordinate $R$.

### Normalization

First, we non-dimensionalize our set of equations. As reference length we choose the particle radius in the Lagrangian frame $R_0$ and as reference time the current dependent cycle time $t_{\mathrm{cycle}}$. Accordingly, the particle center is located at $\tilde{R} = 0$ and the particle-SEI interface at $\tilde{R} = 1$. Table SI-1 summarizes the dimensionless variables of our model. Here, $R_{\mathrm{gas}}$ is the universal gas constant and $c_{\mathrm{Li}^0,\mathrm{ref}}$ is the reference concentration of lithium atoms inside the SEI. The dimensionless chemo-mechanical DAE of our particle-SEI system are listed in

equations SI-42-SI-47.

$$\frac{\mathrm{d}\tilde{c}}{\mathrm{d}\tilde{t}} = \mathrm{Fo}\frac{1}{\tilde{R}^2}\frac{\partial}{\partial\tilde{R}}\tilde{R}^2\left(\frac{\partial\tilde{\mu}}{\partial\tilde{c}}\right)^{-1}\frac{\partial\tilde{\mu}}{\partial\tilde{R}} \tag{SI-42}$$

$$0 = \frac{\partial}{\partial\tilde{R}}\tilde{P}_R - \frac{2}{\tilde{R}}\left(\tilde{P}_\theta - \tilde{P}_R\right) \tag{SI-43}$$

$$\frac{\mathrm{d}\left(\epsilon_{\mathrm{SEI}}c_{\mathrm{Li}^0,0}\right)}{\mathrm{d}\tilde{t}} = \mathrm{Fo}_{\mathrm{SEI}}\frac{1}{\tilde{R}^2}\epsilon_{\mathrm{SEI}}\frac{\partial}{\partial\tilde{R}}\tilde{R}^2\frac{\partial(\tilde{c}_{\mathrm{Li}^0,0})}{\partial\tilde{R}} - 2\tilde{r}_{\mathrm{SEI},0} \tag{SI-44}$$

$$\frac{\mathrm{d}\varepsilon_{\mathrm{SEI}}}{\mathrm{d}\tilde{t}} = \tilde{r}_{\mathrm{SEI},0}\tilde{V} \tag{SI-45}$$

$$0 = \frac{\partial}{\partial\tilde{R}}\tilde{P}_{\mathrm{SEI},R} - \frac{2}{\tilde{R}}\left(\tilde{P}_{\mathrm{SEI},\theta} - \tilde{P}_{\mathrm{SEI},R}\right) \tag{SI-46}$$

$$\frac{\mathrm{d}}{\mathrm{d}\tilde{t}}\bar{\mathbf{F}}_{\mathrm{pl}} = \tilde{\phi}\left(3\tilde{\mathbf{M}}_{\mathrm{c}}^{\mathrm{dev}} + \xi\sinh\left(\mathrm{tr}\,\tilde{\mathbf{M}}_{\mathrm{c}}/2\right)\right)\bar{\mathbf{F}}_{\mathrm{pl}}. \tag{SI-47}$$

The dimensionless first Piola–Kirchhoff stress inside the particle $\tilde{\mathbf{P}}$ and the SEI $\tilde{\mathbf{P}}_{\mathrm{SEI}}$ depend on elastic deformations $\mathbf{F}_{\mathrm{el}}$ according to Equations SI-22 and SI-37. Over time the SEI grows according to the dimensionless reaction rate $\tilde{r}_{\mathrm{SEI},0}$, defined by

$$\tilde{r}_{\mathrm{SEI},0} = \frac{1}{\bar{J}}\mathrm{Fo}_{\mathrm{SEI}}\mathrm{Da}\tilde{A}_{\mathrm{v}}\tilde{c}^2_{\mathrm{Li}^0,0}. \tag{SI-48}$$

**Initial and Boundary Conditions**

We close our DAE system by defining initial and boundary conditions. Initially, the particle has a homogeneous lithium concentration $\tilde{c}(\tilde{R},0) = \tilde{c}_0(U_{0,0})$. Over time, this concentration changes due to a constant external flux at the particle SEI boundary $\tilde{N}(1,\tilde{t}) = \tilde{N}_{\mathrm{ext}} = \pm 1/3$, which is positive for deintercalation and negative for intercalation. At the particle center, we implement symmetry boundary conditions, this means $\tilde{N}(0,\tilde{t}) = 0$ and $\tilde{r}(0,\tilde{t}) = 0$. We couple electrode and SEI mechanically by stating geometrical and mechanical continuity with the two boundary conditions

$$\tilde{r}(1,\tilde{t})|_- = \tilde{r}(1,\tilde{t})|_+, \qquad P_R(1,\tilde{t})|_- = P_R(1,\tilde{t})|_+. \tag{SI-49}$$

The SEI expands freely into the electrolyte so that the radial stress vanishes at the maximum radius of the SEI-electrolyte domain $\sigma_R(\tilde{R}_{\mathrm{SEI,max}},\tilde{t}) = 0$.

To determine the interstitial concentration, we rely on the long-term limit of our model developed in 14. This yields the following equation for the lithium atom concentration at the electrode-SEI interface

$$\tilde{c}_{\mathrm{Li}^0,0}(1,\tilde{t}) = \exp\left(\tilde{\mu}(1,\tilde{t}) - \tilde{\eta}_{\mathrm{int}} - \tilde{\mu}_{\mathrm{Li}^0,0}\right) \tag{SI-50}$$

which depends on the chemical potential $\tilde{\mu}$ of lithium inside the electrode, Equation SI-23, and the reference chemical potential for lithium atoms inside the SEI $\tilde{\mu}_{\mathrm{Li}^0,0}$. To determine the dimensionless intercalation overpotential, we use

a symmetric Butler-Volmer approach $\tilde{\eta}_{\text{int}} = 2\,\text{asinh}\left(j_{\text{int}}/(2j_{\text{int},0}\sqrt{\tilde{c}})\right)$ with the intercalation current density $j_{\text{int}}$ and the exchange current density $j_{\text{int},0}$. For the SEI porosity, we prescribe a dual layer starting profile $\epsilon_{\text{SEI}}(\tilde{R}, 0)$ motivated by experimental findings [28, 29] and the SEI model of Single *et al.* [11, 12].

# 2 Computational Details

## 2.1 Implementation

We numerically solve the DAE SI-42-SI-47 with the boundary and initial conditions described in the previous section. To this aim, we transform the partial differential equations (PDE) to ordinary differential equations (ODE) by discretizing the radial dimension with a finite difference scheme. We solve the resulting ODE in time with the implicit ODE solver ode15i of MATLAB. As stopping criteria for the simulation, we prescribe a maximum anode potential $U_{\text{max}}$ for discharging and a minimum anode potential $U_{\text{min}}$ for charging.

The SEI plasticity and fracture introduce discontinuities in our physical system. To overcome the numerical challenges, we introduce three distinct stages of SEI mechanics: elastically deforming, plastically deforming, and broken. Initially, we locally label the SEI as elastically deforming ($\xi(\epsilon_{\text{elyt},0}) < 1$) or broken ($\xi(\epsilon_{\text{elyt},0}) = 1$), based on Equation SI-39. Elastically deforming SEI elements exhibit no plastic flow, which mathematically results from the Karush-Kuhn-Tucker-condition leading to $\tilde{\phi} = 0$. Upon reaching the yield limit $f = 0$, the SEI locally transitions to the plastic regime and deforms plastically with $\tilde{\phi} > 0$. During deformation, the SEI pores expand until the SEI eventually breaks at $\xi(\epsilon_{\text{elyt}} \geq \epsilon_{\text{elyt,frac}}) = 1$ and is switched to broken. For broken parts of the SEI, the yield function SI-38 dictates $\sigma = 0$. Hence, the momentum balance SI-46 is trivially fulfilled and we need another equation to determine the deformation of these elements. To this aim, we assume free expansion/contraction, *e.g.* the deformation rate $\dot{r}_i$ of the broken SEI element $i$ is equal to the deformation rate of the adjacent element $\dot{r}_i = \dot{r}_{i-1}$.

SEI growth and mechanical compression decrease the SEI porosity below the fracture porosity and thus lead to healing of broken SEI elements. In this case, we transition the SEI element state from broken to elastically deforming and set the current deformation of this element to be the new reference deformation $\mathbf{F}_{\text{ref}}$. Thereby, the healed element starts in a stress free state.

## 2.2 Parameter

In this subsection, we list the model parameters in table SI-2.

| Name | Parameter | Value | Source |
|---|---|---|---|
| Universal gas constant | $R_{\text{gas}}$ | $8.314\,\text{J}\,\text{mol}^{-1}\,\text{K}^{-1}$ | |
| Faraday constant | $F$ | $96\,485\,\text{C}\,\text{mol}^{-1}$ | |

| | | | |
|---|---|---|---|
| Temperature | $T$ | 298.15 K | |
| | | Silicon | |
| Particle Radius | $R_{\max}$ | 50 nm | [10] |
| Diffusivity of lithium | $D_{\mathrm{Li}}$ | $1 \times 10^{-17}\,\mathrm{m^2\,s^{-1}}$ | [30] |
| Maximum lithium concentration | $c_{\mathrm{Li,max}}$ | $311.47 \times 10^{3}\,\mathrm{mol\,m^{-3}}$ | [30] |
| Molar volume of lithium | $v$ | $10.96 \times 10^{-6}\,\mathrm{m^3\,mol^{-1}}$ | [31] |
| Young's modulus | $E_{\mathrm{Si}}$ | 90.13 GPa | [32] |
| Poisson's ratio | $\nu_{\mathrm{Si}}$ | 0.22 | [32] |
| OCV-Curve | $U_0(\tilde{c})$ | Equation SI-51 | [10] |
| Exchange current density | $j_{\mathrm{int},0}$ | $0.4207\,\mathrm{A\,m^{-2}}$ | [30] |
| | | SEI | |
| Initial SEI thickness | $L_{\mathrm{SEI},0}$ | 25 nm | Assumed |
| SEI domain size | $L_{\max}$ | 40 nm | |
| Diffusivity of lithium inside the SEI | $D_{\mathrm{Li},0}$ | $1 \times 10^{-15}\,\mathrm{m^2\,s^{-1}}$ | [13] |
| Lithium atom reference concentration | $c_{\mathrm{Li,0,ref}}$ | $1 \times 10^{-3}\,\mathrm{mol\,m^{-3}}$ | [13] |
| Lithium stoichiometry of reaction 6 | $\nu_{\mathrm{SEI}}$ | 2 | |
| Typical SEI pore edge length | $a_0$ | 1 nm | [11, 12] |
| SEI Surface site density | $\Gamma$ | $4 \times 10^{-6}\,\mathrm{mol\,m^{-2}}$ | [11, 12] |
| SEI molar volume | $\bar{V}_{\mathrm{SEI}}$ | $96.2 \times 10^{-6}\,\mathrm{m^3\,mol^{-1}}$ | [12, 33] |
| Electrolyte molar volume | $\bar{V}_{\mathrm{EC}}$ | $66.7 \times 10^{-6}\,\mathrm{m^3\,mol^{-1}}$ | [12, 34] |
| Rate constant of reaction 6 | $k$ | $1 \times 10^{2}\mathrm{m^6 mol^{-2} s^{-1}}$ | Fitted, Figure 3 [9] |
| Lithium atom reference chemical potential | $\mu_{\mathrm{Li^0},0}$ | $-9.7\,\mathrm{kJ\,mol^{-1}}$ | Fitted, Figure 3 [9] |
| Inner SEI thickness | $L_{\mathrm{SEI,inner}}$ | 5 nm | Fitted, Figure 4 [35] |
| SEI transition length | $L_{\mathrm{trans}}$ | 10 nm | Fitted, Figure 4 [35] |
| Inner SEI porosity | $\epsilon_{\mathrm{elyt,min,inner}}$ | 0.01 | Fitted, Figure 4 [35] |
| Outer SEI porosity | $\epsilon_{\mathrm{elyt,min,outer}}$ | 0.2 | Fitted, Figure 4 [35] |
| Fracture porosity | $\epsilon_{\mathrm{elyt,crit}}$ | 0.25 | Fitted, Figure 4 [35] |
| Inner Young's modulus | $E_{\mathrm{SEI,inner}}$ | 900 MPa | Fitted, Figure 4 [35] |
| Outer Young's modulus | $E_{\mathrm{SEI,outer}}$ | 180 MPa | Fitted, Figure 4 [35] |
| Inner yield stress | $\sigma_{\mathrm{Y,inner}}$ | 49.5 MPa | Fitted, Figure 4 [35] |
| Outer yield stress | $\sigma_{\mathrm{Y,outer}}$ | 9.9 MPa | Fitted, Figure 4 [35] |
| Poisson's ratio | $\nu_{\mathrm{SEI}}$ | 0.5 | Incompressible matrix |
| | | Chemical Parametrization | |
| Initial SEI thickness | $L_{\mathrm{SEI},0}$ | 15 nm | Fitted, Figure 3 [9] |
| SEI domain size | $L_{\max}$ | 60 nm | |
| Temperature | $T$ | 323.15 K | [9] |

| | | | |
|---|---|---|---|
| Anode surface area | $A_{el}$ | $14.24\,m^2$ | [9, 13] |
| Anode maximum capacity | $Q_{max}$ | 10 080 C | [9, 13] |
| Linear SoH loss | $\Delta SoH_{lin}$ | 4.5 % | [13] |
| Mechanical Parametrization | | | |
| Particle Radius | $R_{max}$ | 11.15 µm | [35] |
| Initial SEI thickness | $L_{SEI,0}$ | 100 nm | [35] |
| SEI domain size | $L_{max}$ | 200 nm | |

Table SI-2: Model parameter

Equation SI-51 shows the OCV-curve for silicon [10].

$$U_0(\tilde{c}) = \frac{-0.2453\tilde{c}^3 - 0.00527\tilde{c}^2 + 0.2477\tilde{c} + 0.006457}{\tilde{c} + 0.002493} \tag{SI-51}$$

# 3 Dividing the Deformation in reversible and irreversible Parts

In this section, we show the transformation of mechanical power density into reversible and irreversible parts. We start by transforming the contraction $\mathbf{P}:\dot{\mathbf{F}}$ to the change of right Cauchy-Green tensor $\dot{\mathbf{C}}$. For this we use the identity $\mathbf{C} = \mathbf{F}^{\mathsf{T}}\mathbf{F}$ and apply the product rule to obtain $\dot{\mathbf{F}} = \frac{1}{2}\mathbf{F}^{-\mathsf{T}}\dot{\mathbf{C}}$. Inserting this into the contraction $\mathbf{P}:\dot{\mathbf{F}}$ with the identity $\mathbf{A}:(\mathbf{B}\mathbf{D}) = (\mathbf{B}^{\mathsf{T}}\mathbf{A}):\mathbf{D}$ leads to $\frac{1}{2}\mathbf{T}:\dot{\mathbf{C}}$ with the second Piola-Kirchhoff stress $\mathbf{T} = \mathbf{F}^{-1}\mathbf{P}$.

Based on this expression, we now proceed to subdivide the deformation tensor into a plastic and a reversible part $\mathbf{F} = \mathbf{F}_{rev}\mathbf{F}_{pl}$. Note here that the tensor product is not commutative so that our ordering implies that the geometry is first plastically then reversibly deformed. This leads to the following expression for the temporal change of the right Cauchy-Green tensor

$$\mathbf{C} = \mathbf{F}_{pl}^{\mathsf{T}}\mathbf{C}_{rev}\mathbf{F}_{pl} \tag{SI-52}$$

$$\dot{\mathbf{C}} = \mathbf{F}_{pl}^{\mathsf{T}}\left(\dot{\mathbf{C}}_{rev} + 2\mathbf{C}_{rev}\mathbf{L}_{pl}\right)\mathbf{F}_{pl}. \tag{SI-53}$$

Here we additionally assumed that the plastic deformation is free of rotations, so that its velocity gradient is symmetric $\mathbf{L}_{pl} = \mathbf{L}_{pl}^{\mathsf{T}}$. Similarly, the reversible Cauchy-Green tensor is by definition symmetric $\mathbf{C}_{rev} = \mathbf{F}_{rev}^{\mathsf{T}}\mathbf{F}_{rev} = \mathbf{C}_{rev}^{\mathsf{T}}$. Next we insert this rate of deformation into the mechanical power density

$$\frac{1}{2}\mathbf{T}:\dot{\mathbf{C}} = \frac{1}{2}\mathbf{T}_{rev}:\dot{\mathbf{C}}_{rev} + \mathbf{M}:\mathbf{L}_{pl}. \tag{SI-54}$$

Here we used the tensor identity $\mathbf{A}:(\mathbf{B}\mathbf{D}) = (\mathbf{A}\mathbf{D}^{\mathsf{T}}):\mathbf{B}$ to transform the second Piola-Kirchhoff stress to its reversible counterpart $\mathbf{T}_{rev} = \mathbf{F}_{pl}\mathbf{T}\mathbf{F}_{pl}^{\mathsf{T}}$. Additionally we introduced the Mandel stress $\mathbf{M} = \mathbf{C}_{rev}\mathbf{T}_{rev}$ as conjugate stress to the plastic deformation rate $\mathbf{L}_{pl} = \dot{\mathbf{F}}_{pl}\mathbf{F}_{pl}^{-1}$.

# 4 Deriving an expression for the specific surface

We determine the specific surface $A_\mathrm{V}$ with the finite cube approach developed by Single *et al.* [11, 12] and adapt it to a spherical geometry. Consider a spherical electrolyte segment of size $\mathrm{d}V = a_0^3$ with the edges $a_0 = \mathrm{d}R = R\sin(\theta)\mathrm{d}\phi = R\mathrm{d}\theta$. At each side, the electrolyte segment adjoins to an SEI element with the chance $\epsilon_\mathrm{SEI}$ of the respective element. We assume a constant porosity in circumferential direction, so that the porosity varies only in radial direction. Summing up over all surface elements along with their probability to contain electrolyte yields

$$\begin{aligned}\sum A_i =& \epsilon_\mathrm{SEI}\left(2R\mathrm{d}\theta\mathrm{d}R + 2R\sin(\theta)\mathrm{d}\phi\mathrm{d}R\right)\\ &+ \epsilon_\mathrm{SEI}(R-\mathrm{d}R)\left(R-\frac{\mathrm{d}R}{2}\right)^2\sin(\theta)\mathrm{d}\phi\mathrm{d}\theta\\ &+ \epsilon_\mathrm{SEI}(R+\mathrm{d}R)\left(R+\frac{\mathrm{d}R}{2}\right)^2\sin(\theta)\mathrm{d}\phi\mathrm{d}\theta.\end{aligned} \tag{SI-55}$$

With the edge length $a_0$ of the spherical segment, we simplify the first term to $\epsilon_\mathrm{SEI}\left(2R\mathrm{d}\theta\mathrm{d}R + 2R\sin(\theta)\mathrm{d}\phi\mathrm{d}R\right) = 4\epsilon_\mathrm{SEI}a_0^2$. In the radial direction, we use a Taylor series up to second order to approximate the change of porosity

$$\begin{aligned}\epsilon_\mathrm{SEI}(R+\mathrm{d}R) &= \epsilon_\mathrm{SEI} + \mathrm{d}R\frac{\mathrm{d}\epsilon_\mathrm{SEI}}{\mathrm{d}R} + \frac{\mathrm{d}R^2}{2}\frac{\mathrm{d}^2\epsilon_\mathrm{SEI}}{\mathrm{d}R^2}\\ \epsilon_\mathrm{SEI}(R-\mathrm{d}R) &= \epsilon_\mathrm{SEI} - \mathrm{d}R\frac{\mathrm{d}\epsilon_\mathrm{SEI}}{\mathrm{d}R} + \frac{\mathrm{d}R^2}{2}\frac{\mathrm{d}^2\epsilon_\mathrm{SEI}}{\mathrm{d}R^2}.\end{aligned} \tag{SI-56}$$

Combining equations SI-55 and SI-56 leads to

$$\begin{aligned}\sum A_i =& 4\epsilon_\mathrm{SEI}a_0^2 + \left(\epsilon_\mathrm{SEI} + \mathrm{d}R\frac{\mathrm{d}\epsilon_\mathrm{SEI}}{\mathrm{d}R} + \frac{\mathrm{d}R^2}{2}\frac{\mathrm{d}^2\epsilon_\mathrm{SEI}}{\mathrm{d}R^2}\right)\\ &\cdot\left(R^2 + R\mathrm{d}R + \frac{\mathrm{d}R^2}{4}\right)\sin(\theta)\mathrm{d}\phi\mathrm{d}\theta\\ &+\left(\epsilon_\mathrm{SEI} - \mathrm{d}R\frac{\mathrm{d}\epsilon_\mathrm{SEI}}{\mathrm{d}R} + \frac{\mathrm{d}R^2}{2}\frac{\mathrm{d}^2\epsilon_\mathrm{SEI}}{\mathrm{d}R^2}\right)\\ &\cdot\left(R^2 - R\mathrm{d}R + \frac{\mathrm{d}R^2}{4}\right)\sin(\theta)\mathrm{d}\phi\mathrm{d}\theta\\ \sum A_i =& \mathcal{O}(\mathrm{d}R^3) + 4\epsilon_\mathrm{SEI}a_0^2 + \sin(\theta)\mathrm{d}\phi\mathrm{d}\theta\\ &\cdot\left[2\epsilon_\mathrm{SEI}R^2 + R^2\mathrm{d}R^2\frac{\mathrm{d}^2\epsilon_\mathrm{SEI}}{\mathrm{d}R^2} + \epsilon_\mathrm{SEI}\frac{\mathrm{d}R^2}{2} + 2R\mathrm{d}R^2\frac{\mathrm{d}\epsilon_\mathrm{SEI}}{\mathrm{d}R}\right]\\ \sum A_i =& 6\epsilon_\mathrm{SEI}a_0^2 + a_0^4\left(\frac{1}{2R^2}\epsilon_\mathrm{SEI} + \frac{2}{R}\frac{\mathrm{d}\epsilon_\mathrm{SEI}}{\mathrm{d}R} + \frac{\mathrm{d}^2\epsilon_\mathrm{SEI}}{\mathrm{d}R^2}\right).\end{aligned} \tag{SI-57}$$

We obtain the specific surface $A_\mathrm{V}$ of an electrolyte element from the last expression by dividing by the volume $a_0^3$ of the element and multiplying by the

fraction of electrolyte elements $\epsilon_{\mathrm{elyt}}$.

$$A_{\mathrm{V}} = \frac{6}{a_0}\epsilon_{\mathrm{elyt}}\left[\epsilon_{\mathrm{SEI}} + \frac{a_0^2}{6}\left(\frac{\mathrm{d}^2\epsilon_{\mathrm{SEI}}}{\mathrm{d}R^2} + \frac{2}{R}\frac{\mathrm{d}\epsilon_{\mathrm{SEI}}}{\mathrm{d}R} + \frac{1}{2R^2}\epsilon_{\mathrm{SEI}}\right)\right] \tag{SI-58}$$

## References


[1] G. A. Holzapfel. *Nonlinear Solid Mechanics.* John Wiley & Sons, Ltd., Chichester, 2000.

[2] A. Latz and J. Zausch. Thermodynamic consistent transport theory of Li-ion batteries. *J. Power Sources*, 196(6):3296–3302, 2011.

[3] A. Latz and J. Zausch. Multiscale modeling of lithium ion batteries: Thermal aspects. *Beilstein J. Nanotechnol.*, 6(1):987–1007, apr 2015.

[4] M. Schammer, B. Horstmann, and A. Latz. Theory of Transport in Highly Concentrated Electrolytes. *J. Electrochem. Soc.*, 2021.

[5] J. Mandel. *Plasticite classique et viscoplasticite:.* CISM International Centre for Mechanical Sciences. Springer, 1972.

[6] J. Lubliner. Plasticity Revised Edition. *J. Appl. Mech.*, 59(1):540, 2006.

[7] G. F. Castelli, L. von Kolzenberg, B. Horstmann, A. Latz, and W. Dörfler. Efficient simulation of chemical-mechanical coupling in battery active particles. *Energy Technol.*, 2021.

[8] A. Latz and J. Zausch. Thermodynamic derivation of a Butler-Volmer model for intercalation in Li-ion batteries. *Electrochim. Acta*, 110:358–362, 2013.

[9] P. Keil, S. F. Schuster, J. Wilhelm, J. Travi, A. Hauser, R. C. Karl, and A. Jossen. Calendar Aging of Lithium-Ion Batteries. *J. Electrochem. Soc.*, 163(9):A1872–A1880, 2016.

[10] C. K. Chan, H. Peng, G. Liu, K. McIlwrath, X. F. Zhang, R. A. Huggins, and Y. Cui. High-performance lithium battery anodes using silicon nanowires. *Nat. Nanotechnol.*, 3(1):31–35, 2008.

[11] F. Single, B. Horstmann, and A. Latz. Dynamics and morphology of solid electrolyte interphase (SEI). *Phys. Chem. Chem. Phys.*, 18(27):17810–17814, 2016.

[12] F. Single, B. Horstmann, and A. Latz. Revealing SEI Morphology: In-Depth Analysis of a Modeling Approach. *J. Electrochem. Soc.*, 164(11):E3132–E3145, 2017.

[13] F. Single, A. Latz, and B. Horstmann. Identifying the Mechanism of Continued Growth of the Solid–Electrolyte Interphase. *ChemSusChem*, 11(12):1950–1955, 2018.

[14] L. von Kolzenberg, A. Latz, and B. Horstmann. Solid–Electrolyte Interphase During Battery Cycling: Theory of Growth Regimes. *ChemSusChem*, 13(15):3901–3910, 2020.

[15] S. Shi, Y. Qi, H. Li, and L. G. Hector. Defect Thermodynamics and Diffusion Mechanisms in $Li_2CO_3$ and Implications for the Solid Electrolyte Interphase in Li-Ion Batteries. *J. Phys. Chem. C*, 117(17):8579–8593, 2013.

[16] F. A. Soto, Y. Ma, J. M. Martinez De La Hoz, J. M. Seminario, and P. B. Balbuena. Formation and Growth Mechanisms of Solid-Electrolyte Interphase Layers in Rechargeable Batteries. *Chem. Mat.*, 27(23):7990–8000, 2015.

[17] J. Newman and K. E. Thomas-Alyea. *Electrochemical systems*. John Wiley & Sons, 2012.

[18] M. Danielsson, D. M. Parks, and M. C. Boyce. Constitutive modeling of porous hyperelastic materials. *Mech. Mater.*, 36(4):347–358, 2004.

[19] A. L. Gurson. Continuum theory of ductile rupture by void nucleation and growth: Part I—Yield criteria and flow rules for porous ductile media. *J. Eng. Mater. Technol. Trans. ASME*, 99:2–15, 1977.

[20] V. Tvergaard. Influence of voids on shear band instabilities under plane strain conditions. *Int. J. Fract.*, 17(4):389–407, 1981.

[21] V. Tvergaard. Influence of void nucleation on ductile shear fracture at a free surface. *J. Mech. Phys. Solids*, 30(6):399–425, 1982.

[22] V. Tvergaard and A. Needleman. Analysis of the cup-cone fracture in a round tensile bar. *Acta Metall.*, 32(1):157–169, 1984.

[23] F. Reusch, B. Svendsen, and D. Klingbeil. Local and non-local Gurson-based ductile damage and failure modelling at large deformation. *Eur. J. Mech. A Solids*, 22(6):779–792, 2003.

[24] R. von Mises. Mechanik der plastischen Formänderung von Kristallen. *J. Appl. Math. Mech.*, 8(3):161–185, 1928.

[25] R. Hill. A variational principle of maximum plastic work in classical plasticity. *Q. J. Mech. Appl. Math.*, 1(October):18–28, 1947.

[26] R. Hill. On the state of stress in a plastic-rigid body at the yield point. *Philos. Mag.*, 42(331):868–875, 1951.

[27] G. Taylor. A connexion between the criterion of yield and the strain ratio. *Proc. R. Soc. Lond. A Math. Phys. Sci.*, 191(1027):441–446, 1947.

[28] K. Edström, M. Herstedt, and D. P. Abraham. A new look at the solid electrolyte interphase on graphite anodes in Li-ion batteries. *J. Power Sources*, 153(2):380–384, 2006.

[29] E. Peled and S. Menkin. Review—SEI: Past, Present and Future. *J. Electrochem. Soc.*, 164(7):A1703–A1719, 2017.

[30] A. Verma, A. A. Franco, and P. P. Mukherjee. Mechanistic Elucidation of Si Particle Morphology on Electrode Performance. *J. Electrochem. Soc.*, 166(15):A3852–A3860, 2019.

[31] M. N. Obrovac and L. J. Krause. Reversible Cycling of Crystalline Silicon Powder. *J. Electrochem. Soc.*, 154(2):A103, 2007.

[32] V. B. Shenoy, P. Johari, and Y. Qi. Elastic softening of amorphous and crystalline Li-Si Phases with increasing Li concentration: A first-principles study. *J. Power Sources*, 195(19):6825–6830, 2010.

[33] O. Borodin, G. D. Smith, and P. Fan. Molecular dynamics simulations of lithium alkyl carbonates. *J. Phys. Chem. B*, 110(45):22773–22779, 2006.

[34] R. Naejus, D. Lemordant, R. Coudert, and P. Willmann. Excess thermodynamic properties of binary mixtures containing linear or cyclic carbonates as solvents at the temperatures 298.15 K and 315.15 K. *J. Chem. Thermodyn.*, 29(12):1503–1515, 1997.

[35] I. Yoon, S. Jurng, D. P. Abraham, B. L. Lucht, and P. R. Guduru. Measurement of mechanical and fracture properties of solid electrolyte interphase on lithium metal anodes in lithium ion batteries. *Energy Storage Mater.*, 25:296–304, 2020.
